# Supplementary material for: Differentially-Private Hierarchical Clustering with Provable Approximation Guarantees
Source: arXiv:2302.00037 source file (2023-05-23)
Supplement: Supplementary file 1 [file appendix_old.tex]

\section{Ale: Back of the envelope calculation on the efficacy of Vu's method + JL}

Consider the paper of Vu "A SIMPLE SVD ALGORITHM FOR FINDING HIDDEN PARTITIONS", in this section we give back of the envelope calculations that suggest that private JL over SVD will work only if the graph has $> \sqrt n$ degree. However, in this case, it seems that the black box algorithm is near optimal at least for constant many communities.  

Let $A$ be the matrix where $A_{ij}$ is the probability of i and j being connected. Let $\hat{A}$ be the sampled graph we receive.

Let $\Delta = ||A_u-A_v||$ be the distance of two columns for vectors in two distinct clusters. 

Let $\hat{P^k}$ be the projection matrix we obtain from the top k singular vectors of $\hat{A}$ 

Vu (and others) shows the following results.
\begin{fact}
Let $\hat{p_u} = \hat{P^k} \hat{A}_u$ be the projection of the u-th column into this space.

Under some conditions on p,q,s,n, we have that
$$||\hat{p}_u - A_u|| < \Delta / 12$$
and hence for $u,v$ in the same cluster
$$||\hat{p}_u - \hat{p}_v || < \Delta / 6$$
and
$$||\hat{p}_u - \hat{p}_v || > 5 \Delta  / 6$$
\end{fact}

This means we can reconstruct the clusters exactly \textbf{ only if estimate the distances of projected points an additive error less } than around $\Delta/12$.

Consider the case of two communities of equal size. $k=2$, $s=n/2$ is the size of each community. Let $p,q$ be the intra-, inter- cluster probabilities. let $p=a/n$ and $q=b/n$ for $a,b$ possibly function of n.

$$\Delta = (p-q)\sqrt{n} = (a-b)/\sqrt{n}$$

So if the intra cluster probabilites are $<1/\sqrt{n}$ we have that we need an additive error that is vanishingly small.  

Any DP algorithm that introduces an additive error of even $1$ will not work. Reading the JL paper seems likely that the additive error is $O(w)$ where $w$ is $polylog(n)/\epsilon$.


On the positive side, however, the projection matrix seems to have all small entries (e.g. all entries are < $1/sqrt(n)$), but it is not clear if this helps. 



\section{A Two-Step Approach for Dasgupta's objective}
Here, we design a DP algorithm for computing an HC of $G$. We consider the combination of two algorithms. First, we apply a DP cut-preservation algorithm to obtain a balanced-cut approximation, and then we solve HC assuming an $(a_n, b_n)$-approximation to balanced cut.

In the balanced cut problem, we seek to find a balanced cut $S$ that minimizes the following:
\[
    \phi(G) = \min_{S \subseteq V, \frac{n}{3} \leq |S| \leq \frac{2n}{3}} \frac{w(S,V \setminus S)}{|S||V \setminus S|} 
\]

\begin{defn}
For sequences of positive real numbers $\{a_1, a_2, \ldots\}$ and $\{b_1, b_2, \ldots \}$, 
we say an algorithm $A$ is an $(a_n, b_n)$-approximation to balanced cut if, for all $n$ and $G \in \calG_n$, it outputs a balanced cut $S$ such that 
\[
    \frac{w(S, V \setminus S)}{|S||V \setminus S|} \leq a_n \phi(G) + b_n.
\]
\end{defn}

\subsection{DP balanced cut}

\begin{lem}
There exists a (non-efficient) algorithm $A : \calG_n \rightarrow \calG_n$ satisfies $\epsilon$-edge DP, and for any input graph $G = (V, E, w)$, the following hold with probability $1-o(1)$:
\begin{itemize}
    \item $A(G) = (V, E', w')$ contains $O(n \log n)$ edges.
    \item For any cut $S$, we have $0.9w(S, V \setminus S)  - O(\frac{n \log^2 n}{\epsilon}) \leq w'(S, V \setminus S) \leq 1.1 w(S, V \setminus S) + O(\frac{n \log^2 n}{\epsilon})$.
    \item $A$ is a $(1.1, \frac{\log^2 n}{n})$-approximation to balanced cut.
\end{itemize}
\end{lem}
\begin{proof}
It is a fundamental result that exists a weighted graph $G_1 = (V, E_1, w_1)$ with $C_1 n \log n$ edges such that for any cut $S$, we have $0.9 w_1(S, V \setminus S) \leq w(S, V \setminus S) \leq 1.1 w_1(S, V \setminus S)$ for a constant $C_1 > 0$. However, simply releasing $G_1$ is not private. We consider the exponential mechanism with domain $\calX$ consisting of weighted graphs with $C_1n \log n$ edges with edge weights in $[n]$. We consider such edge weights because this is a discrete domain of size $\binom{n^2}{C_1n \log n} n^{n \log n} \leq n^{3C_1n \log n} \leq e^{4C_1n \log^2 n}$. Let
\[
L(G, H) = \sup_{S \subseteq V} |w_G(S, V \setminus S) - w_H(S, V \setminus S)|.
\]
Observe there is a graph $G_2 \in \calX$ such that $L(G_1, G_2) \leq n$---simply $G_1$ with its edges rounded.

Our exponential mechanism will use the loss function $L_{G_1}(H) = L(G_1, H)$.
This loss function clearly has sensitivity $1$ under our model of differential privacy.
Let $\calY = \{H \in \calX : L_{G_1}(H) \leq  L_{G_1}(G_2) + 9\tfrac{C_1}{\epsilon} n \log^2 n\}$. 
The probability of outputting an element in $\calY$ is at least $\frac{K}{K+M}$, where
\begin{align*}
    K &= \sum_{H \in \calY} e^{-\epsilon L_{G_1}(H)/ 2} \\
    M &= \sum_{H \in \calG_n \setminus \calY} e^{-\epsilon L_{G_1}(H) / 2}
\end{align*}
Because $G_2 \in \calY$, we have $K \geq e^{-\epsilon L_{G_1}(G_2) / 2}$ and 
\begin{align*}
    M &\leq |\calX| e^{-\epsilon (L_{G_1}(G_2) + 9\tfrac{C_1}{\epsilon} n \log^2 n)/ 2} \\
    &\leq e^{4C_1n \log^2 n}e^{-\epsilon L_{G_1}(G_2)/2} e^{-4.5C_1 n \log^2 n} \\
    &\leq e^{-\epsilon L_{G_1}(G_1)/2} e^{-n}.
\end{align*}
Thus, the probability of releasing an element in $X$ is at least $\frac{1}{1 + e^{{-n}}} = 1 - o(1)$. Assuming this event happens, we have
\[
    L(G_1, A(G)) \leq L(G_1, G_2) + \frac{9C_1}{\epsilon} n \log^2 n \leq \frac{10C_1}{\epsilon} n \log^2 n.
\]
Thus, $w_1(S, V \setminus S) - \frac{10C_1}{\epsilon} n \log^2 n \leq w_{A(G)} (S, V \setminus S) \leq w_1(S, V \setminus S) + \frac{10C_1}{\epsilon} n \log^2 n$, and we obtain the desired result.

\end{proof}

We apply the result of Elias et. al.
\begin{prop}
    There exists a polynomial-time algorithm which releases a graph $G' = (V, E, w')$ such that for all cuts $S$, we have
    \[
        |w(S, V \setminus S) - w'(S, V \setminus S) | \leq n^{3/2}\log(\frac{n}{\epsilon})^2.
    \]
\end{prop}
This provides the following corollary:
\begin{coro}
There exists a polynomial-time algorithm which is a $(\log n, \tilde{O}(\frac{1}{\sqrt{n}}))$-approximation to balanced cut which satisfies $(\epsilon, \delta)$-DP.
\end{coro}
\begin{proof}
The algorithm runs a $(\log n, 0)$-balanced cut on $G'$ and releases a cut $S'$. Let $S_*$ be the optimal cut in $G$. We are guaranteed that:
\[
    \frac{w'(S_*, V \setminus S_*)}{|S_*| |V \setminus S_*|} \leq \frac{w(S_*, V \setminus S_*) + n^{3/2} \log (\frac{n}{\epsilon})^2}{|S_*| |V \setminus S_*|} \leq \frac{w(S_* V \setminus S_*)}{|S_*||V \setminus S_*|} + \frac{9 \log(\frac{n}{\epsilon})^2}{2\sqrt{n}}.
\]
The balanced cut algorithm guarantees that the cut $S'$ satisfies
\[
\frac{w'(S', V \setminus S')}{|S'| |V \setminus S'|} \leq \log n \frac{w'(S_*', V \setminus S_*')}{|S_*'||V \setminus S_*'|},
\]
where $S_*'$ is the optimal balanced cut on $G'$. Combining these two observations, we obtain
\[
    \frac{w'(S', V \setminus S')}{|S'| |V \setminus S'|} \leq \log n \frac{w(S_* V \setminus S_*)}{|S_*||V \setminus S_*|} + \frac{9 \log(\frac{n}{\epsilon})^3}{2\sqrt{n}}.
\]
\end{proof}

\subsection{HC from balanced cut}
Here, we make approximation guarantees on HC given an approximation to balanced cut. First, we will introduce a lemma of Dasgupta:

\begin{lem}
Let $G \in \calG_n$ and $T \in \calT_n$ be arbitrary. There exists a subset $S \subset V$ of $T$ such that $\frac{|V|}{3} \leq |S| \leq \frac{2|V|}{3}$, and
\[
    \frac{w(S, V \setminus S)}{|S||V \setminus S|} \leq \frac{27}{4n^3} \dcost_G(T).
\]
\end{lem}

Armed with this lemma, we can show that by picking an $(a_n, b_n)$-approximation to balanced cut, we are able to find an approximation to HC.

\begin{thm}
Let $n$ be fixed, and suppose we pick $T$ with a recursive strategy, selecting a balanced subset of vertices $S$ according to an $(a, b)$ cut approximation. The resulting tree is a $(\frac{27a}{4}\log n, \frac{9b}{4}n \log n)$-approximation to HC.
\end{thm}
\Jnote{TODO: get rid of the $\log n$ factor using Vincent's HC paper.}
\begin{proof}
We will prove the result by induction on $n$. The base case of $n=1$ is trivial.
Suppose for all $i < n$, the algorithm is a $(c_i, d_i)$-approximation to HC, where $c_i = \frac{27a}{4} \log i$, 
$d_i = \frac{9b}{4} i \log i$.
Let $T^*$ be the tree that optimizes $\dcost_G(T)$. Let $S^*$ be the balanced cut optimizing $\phi(G)$. By the lemma, we have
\[
\frac{w(S^*, V \setminus S^*)}{|S^*||V \setminus S^*|} \leq \frac{27}{4 n^3}\dcost_G(T^*).
\]
The algorithm is able to find a balanced cut $S$ such that $w(S, V \setminus S) \leq aw(S^*, V \setminus S^*) + b$. This implies
\[
    \frac{w(S, V \setminus S)}{n^2/4} \leq a\frac{w(S^*, V \setminus S^*)}{|S^*||V \setminus S^*|} + b\frac{9}{2n^2}. 
\]
Because $S,S^*$ are balanced, we obtain $\frac{w(S, V \setminus S)}{n^2/4} \leq \frac{27 a}{4n^3}\dcost_G(T^*) + \frac{9b}{2n^2}$, which implies
\[
    w(S, V \setminus S) \leq a \frac{27}{16n}\dcost_G(T^*) + \frac{9b}{8}.
\]

Let $T = T_1 \cup T_2$ be the output of our HC algorithm. The cost satisfies
\begin{align*}
    \dcost_G(T) \leq n w(S, V \setminus S) + \dcost_{G[S]}(T_1) + \dcost_{G[V \setminus S]}(T_2)
\end{align*}
Let $t_1 = |T_1|$ and $t_2 = |T_2|$. Notice that $t_1 + t_2 = n$, and $\frac{n}{3} \leq t_1, t_2 \leq \frac{2n}{3}$.
Applying the inductive hypothesis on $T_1$, $T_2$, we have 
$\dcost_{G[S]}(T_1) \leq c_{t_1}\dcost_{G[S]}(T_1^*) + d_{t_1}$, and $\dcost_{G[V \setminus S]}(T_2) \leq c_{t_2}\dcost_{G[V \setminus S]}(T_2^*) + d_{t_2}$, where $T_1^*, T_2^*$ are the optimal trees on the subgraph $G[S]$ and $G[V \setminus S]$, respectively. However, because $T^*$ is optimal, we have $\dcost_{G[S]}(T_1^*) + \dcost_{G[V \setminus S]}(T_2^*) \leq \dcost_G(T^*)$, and this gives
\begin{align*}
    \dcost_G(T) &\leq a n\frac{27}{16n}\dcost_G(T^*) + \frac{9b}{8}n + c_{t_1} \dcost_{G[S]}(T_1^*) + d_{t_1} + c_{t_2}\dcost_{G[V \setminus S]}(T_2^*) + d_{t_2} \\
    &\leq \frac{27a}{16} \dcost_G(T^*) + \frac{9b}{8}n + \max\{c_{t_1}, c_{t_2}\} \dcost_{G[S]}(T^*_1) + d_{t_1} + \max\{c_{t_1}, c_{t_2}\}\dcost_{G[V \setminus S]}(T^*_2) + d_{t_2} \\
    &\leq \left(\frac{27a}{16} + \max\{ c_{t_1}, c_{t_2}\} \right) \dcost_G(T^*) + \left(\frac{9b}{8}n + d_{t_1} + d_{t_2}\right) \\
    &\leq a\frac{27}{4}\left(\frac{1}{4} + \max\{ \log(t_1), \log(t_2)\} \right) \dcost_G(T^*) + \frac{9b}{8}\left(n + 2t_1\log(t_1) + 2t_2 \log(t_2) \right)
\end{align*}
For any admissible choice of $t_1, t_2$, we have that $\frac{1}{4} + \max\{ \log(t_1), \log(t_2)\} \leq \log(n) - \log(3/2) < \log(n)$. Furthermore, $t_1 \log(t_1) + t_2 \log (t_2)$ is convex, and is thus maximized at the endpoint $t = \frac{n}{3}$. We have 
\begin{align*}
    n + 2\frac{n}{3} \log(\frac{n}{3}) + 2\frac{2n}{3} \log (\frac{2n}{3}) &\leq n \log n - 2(\log 3) \frac{n}{3} - 2\log (\frac{3}{2}) \frac{2n}{3} + n \\
    &\leq 2n \log n.
\end{align*}
This establishes the inductive hypothesis that
\[
    \dcost_G(T) \leq \frac{27}{4}a \log n \dcost_G(T^*) + \frac{9b}{4}\log n \\
\]
\end{proof}

\begin{coro}
    There is a 
    \begin{itemize}
        \item (Polynomial time): $(\frac{27}{4} (\log n)^2, \frac{9}{4}n^{2.5} \log n(\log \frac{n}{\epsilon})^2)$-approximation to HC that is $(\epsilon, \delta)$-DP.
        \item (Exponential time): $(\frac{27}{4} (\log n)^2, \frac{9}{4}n^2 (\frac{\log^3 n}{\epsilon}))$-approximation to HC that is $(\epsilon, 0)$-DP.
    \end{itemize}
\end{coro}
I suspect we can get rid of some of the $\log$-factors.

\section{Repeating the Analysis for Mosely-Wang objective}
In this section, we use the same two-step approach for $\mwcost$. 

\subsection{DP Max-Uncut Bisection}

\subsection{HC from Max-Uncut Bisection}
\begin{thm}
Given an $(4246, O(n^{2.5}/\epsilon))$-approximation to Max-Uncut Bisection, there is an algorithm which produces a tree which is an $(a_n, n b_n)$-approximation to HC with $\mwcost_G$ for any $G$.
\end{thm}
Recall the algorithm performs max-uncut bisection and then runs average linkage on the two halves.

To prove this theorem, we will recall several important facts from Ahmadian et al.
First, let $T^* = \arg \max_{T \in \calT_n} \mwcost_G(T)$. We split $T$ into subtrees $A, B, C_1, \ldots, C_k$, each of size at most $\frac{n}{2}$, such that $|A \cup B| \geq \frac{n}{2}$ and the tree $T = T_k$, where $T_0 = split(A, B)$ and $T_i = split(C_i, T_{i-1})$. Let $C = C_1 \cup \cdots \cup C_k$. We have the following lemma:

\begin{lem}
    For $T,A,B,C$ defined above, we have $\mwcost_G(T) \leq (\alpha) (n-2) + (\beta) |C|$, where $\alpha = w(A) + w(B) + w(C)$ and $\beta = w(A, B) + w(B,C) + w(A,C)$.
\end{lem}
Now, there are two cases. If $\alpha \leq \beta$, then recall the average linkage tree finds a tree $T$ such that $\mwcost_G(T) \geq \frac{1}{3}(\alpha + \beta)(n-2)$. This means that the average linkage part the Ahmadian et al. algorithm already finds a $\frac{4}{9}$-approximation. 

In the second case, we have the following lemma
\begin{lem}
    For $T, A, B, C$ defined above, suppose $\alpha \geq \beta$. Then, there exists a balanced cut $(L,R)$ of the nodes in $G$ such that the weight of the uncut edges is at least $\alpha - (\alpha-\beta) \delta_{max}(c)$, where $c = \frac{|C|}{n}$ and $\delta_{max}(c) = \frac{c(1-2c)}{1-3c^2}$.
\end{lem}

With these theorems, we can prove our result. Let $L,R$ be the splits of max-uncut.
The revenue generated by our tree is at least
\[
    \mwcost_G(T) \geq (w(L) + w(R))(\frac{1}{3}\left(\frac{n}{2}-2\right) + \frac{n}{2}),
\]
because average linkage is a $\frac{1}{3}$-approximation and there are $\frac{n}{2}$ new nodes added to the cost.
Let $OPT$ be the optimal cost of the max-uncut bisection. We are guaranteed by the previous Lemma that
$OPT \geq \alpha - (\alpha-\beta)\delta_{max}(c)$. Furthermore, $w(L) + w(R) \geq \rho OPT - O(n^{1.5}{\epsilon})$, because we are using a $\rho$-approximation to max-uncut and any cut query is answered within additive factor $\frac{n^{1.5}}{\epsilon}$. Thus,
\[
\mwcost_G(T) \geq (\alpha - (\alpha-\beta)\delta_{max}(c)))\frac{2}{3}\rho (n-1) - \rho\frac{n^{2.5}}{\epsilon}
\]

\subsection{Lower Bound Method 2}
We do this by exhibiting a class of graphs which are a packing with respect to the Dasgupta objective. The class of graph consists of random spanning trees. The following lemma first appeared in~\cite{goyal2009expanders}.

\begin{lem}\label{lem:tree-expander}
Let $T_1, T_2$ be two independent random trees on $n > 100$ vertices. Then, with probability $1-0.8^{n/4}$, $T_1 \cup T_2$ is a $0.1$-vertex expander on all sufficiently large vertex sets. That is, for any $S$ satisfying $\frac{n}{3} \leq S \leq \frac{n}{2}$, we have $|\delta_{T_1 \cup T_2}(S) \setminus S| \geq 0.1 |S|$. 
\end{lem}
\begin{proof}
Our claim fails if there is a balanced cut $S$ and set $S'$ of size $\beta |S|$ disjoint with $S$ such that $\delta_{T_1 \cup T_2}(S) \setminus S \subseteq S'$. We will use a union bound over all possible sets $S, S'$. Suppose $|S| = a$ and without loss of generality, let $S = [a]$ and $S' = \{a+1, \ldots, a+\beta a\}$. Furthermore, due to independence, the probability that both $T_1, T_2$ satisfy $\delta_{T_1 \cup T_2}([a]) \subseteq [a + \beta a]$ is at most the squared probability of $\delta_{T_1}([a]) \subseteq [a + \beta a]$. Thus, the desired probability can be upper bounded by 
\[
    \sum_{a = n/3}^{n/2} \binom{n}{a} \binom{n}{\beta a} \Pr[\delta_{T_1}([a]) \subseteq [a + \beta a]]^2.
\]

Note that $\delta_{T_1}([a]) \subseteq [a + \beta a]$ implies that no edges exist in $T_1$ between $[a]$ and $V \setminus [a + \beta a]$. By negative correlation of edges in a random tree, we have $\Pr[\delta_{T_1}([a]) \subseteq [a + \beta a]] \leq (1-\frac{2}{n})^{a (n-a-\beta a)}$. Thus, our probability is bounded by 
\begin{align*}
    \sum_{a = n/3}^{n/2} \binom{n}{a} \binom{n}{\beta a} \left(1-\frac{2}{n}\right)^{2a (n-a-\beta a)} &\leq \sum_{a = n/3}^{n/2} \left(\frac{en}{a}\right)^a \left(\frac{en}{\beta a}\right)^{\beta a}\left(1-\frac{2}{n}\right)^{2a (n-a-\beta a)} \\
    &\leq n \sup_{\gamma \in [1/3, 1/2]} \left(\frac{e}{\gamma}\right)^{\gamma n} \left(\frac{e}{\beta \gamma}\right)^{\beta \gamma n}\left(1-\frac{2}{n}\right)^{2\gamma n(n-(1+\beta)\gamma n )} \\
    &\leq n \sup_{\gamma \in [1/3, 1/2]} \left(\frac{(e/\gamma)^{1+\beta}}{\beta^\beta}\right)^{\gamma n} e^{-4\gamma (n-(1+\beta)\gamma n )} \\
    &\leq n \sup_{\gamma \in [1/3, 1/2]} \left(\frac{(e/\gamma)^{1+\beta}}{\beta^\beta e^{4(1-(1+\beta)\gamma)}}\right)^{\gamma n}.
\end{align*}
The function $f(\gamma) = \frac{(e/\gamma)^{1+\beta}}{\beta^\beta e^{4(1-(1+\beta)\gamma)}}$ can be written as $\frac{e^{1+\beta}}{\beta^\beta e^4}e^{4(1+\beta) \gamma - (1+\beta) \ln \gamma}$, and thus it is convex in $\gamma$. Thus, it is maximized at $\gamma \in \{\frac{1}{3}, \frac{1}{2}\}$. We have
\begin{align*}
    f(\frac{1}{3}) &= \frac{(3e)^{1+\beta}}{\beta^\beta e^{8/3 - 4\beta/3}} & f(\frac{1}{2}) &= \frac{(2e)^{1+\beta}}{\beta^\beta e^{2-2\beta}}
\end{align*}
When $\beta \rightarrow 0$, we see that $f(\frac{1}{3}) \rightarrow \frac{3}{e^{5/3}} < 0.6$ and $f(\frac{1}{2}) \rightarrow \frac{2}{e} < 0.8$. These inequalities are achieved when $\beta = 0.1$. Thus, the desired probability is at most $n (0.8)^{n/3} < (0.8)^{n/4}$ for $n$ sufficiently large.


\end{proof}
\begin{lem}\label{lem:packing}
For $n > 100$, there exists a set of graphs $G \subseteq \calG_n$ with $|G| = 2^{0.03 n}$ such that for any $G_1, G_2 \in G$, we have for any balanced cut $S$ that $w_{G_1 \cup G_2}(S, V \setminus S) \geq \frac{n}{30}$.
\end{lem}
\begin{proof}
    We generate a set $\calT$ of cardinality $M = 2^{0.03n}$ consisting of trees on $n$ vertices independently at random. By Lemma~\ref{lem:tree-expander}, the probability that the union of any two trees will fail to be a $0.1$-vertex expander on balanced cuts is at most $0.8^{n/4}$. By the union bound, the probability that any two trees in $\calT$ will fail to be a $0.1$-vertex expander is at most $M^2 0.8^{n/4} < 1$, and thus there exists a $\calT$ such that for each $T_1, T_2 \in \calT$, $T_1 \cup T_2$ is a $0.1$-vertex expander on balanced cuts. However, if $T_1 \cup T_2$ is a $0.1$-vertex expander for balanced cuts, then there must be at least $0.1 \frac{n}{3}$ edges crossing the cut, and thus $w_{T_1 \cup T_2}(S, V\setminus S) \geq \frac{n}{30}$.
\end{proof}

\begin{thm}
For any $\epsilon < 0.01$, and any $\epsilon$-edge DP algorithm $A(G)$ which outputs a hierarchical clustering, there is a graph $G$ with $\dcost_G^* \leq O(n \log n)$ such that 
\[
    \E[\dcost_{G}(A(G))] \geq \Omega(n^2).
\]
\end{thm}
\begin{proof}
Let $\calG$ be the set of graphs guaranteed by Lemma~\ref{lem:packing}; namely, $|\calG| = 2^{c_1n}$ and $w_{G \cup G'}(S, V\setminus S) \geq c_2 n$ for any $G, G' \in \calG$ and balanced cut $S$. It clearly holds that $\dcost_G^* \leq O(n \log n)$ for all $G \in \calG$. We claim that any hierarchical clustering $T$ can achieve $\dcost_G(T) \leq \frac{c_2}{4}n^2$ error on at most one $G \in \calG$.

To prove this claim, suppose $T$ achieves $\dcost_G(T) \leq \frac{c_2}{4}n^2$ for some $G$. Let $B$ be the balanced cut of $T$. We know that $\dcost_G(T) \geq w_G(B, V \setminus B) \frac{2n}{3}$. For any other $G' \in \calG$, we also have $\dcost_{G'}(T) \geq w_{G'}(B, V \setminus B) \frac{2n}{3}$. However, we know that
\[
    w_{G'}(B, V \setminus B) + w_{G}(B, V \setminus B) = w_{G' \cup G}(B, V \setminus B) \geq c_2 n.
\]
This implies $\dcost_{G}(T) + \dcost_{G'}(T) \geq \frac{2n}{3}c_2 n$. Thus, $\dcost_{G'}(T) > \frac{c_2}{4}n^2$ for all other $G' \in \calG$. Now, for any $G \in \calG$, define $\calC(G)$ to be those trees $T$ such that $\dcost_G(T) \leq \frac{c_2}{4}n^2$. We have that $\calC(G) \cap \calC(G') = \emptyset$ for all $G,G' \in \calG$.

We prove the theorem using the standard packing argument. Suppose the algorithm $A$ satisfies $\E[\dcost_G(A(G))] \leq \frac{c_2}{8}n^2$ for any $G$. This implies $\Pr[A(G) \notin \calC(G)] \frac{c_2}{4} n^2 \leq \frac{c_2}{8}n^2$, meaning that $\Pr[A(G) \in \calC(G)] \geq \frac{1}{2}$ for all $G \in \calG$. Using the edge DP guarantee up to $2n$ times, this means that $\Pr[A(G) \in \calC(G')] \geq e^{-2n\epsilon} \frac{1}{2}$ for all $G' \in \calG$. Thus,
\begin{align*}
    1 &\geq \Pr[A(G) \in \calC(G)] + \sum_{G' \in \calG, G' \neq G} \Pr[A(G) \in \calC(G')] \\
    &\geq \frac{1}{2} +  (|\calG|-1)e^{-2\epsilon n} \frac{1}{2} \\
    &\geq \frac{1}{2}|\calG|e^{-2\epsilon n} \\
    &\geq 2^{c_1 n - 2\log(e)\epsilon n-1} \\
    &\geq 2^{0.01 n - 1} > 1.
\end{align*}
This is a contradiction, and thus the algorithm $A$ must have higher error.
\end{proof}
\iffalse
\begin{thm}
    For any HC algorithm $A$ which satisfies $\epsilon$-edge DP, there exists a graph $G$ such that
    \[
        \E[\dcost_G(A(G))] \geq \dcost_G^* + O(\frac{n^2}{\epsilon}).
    \]
\end{thm}
We will prove this by supposing the contrary, and deriving a contradiction. Thus, assume that there is an algorithm which achieves for all graphs $G$, $\E[\dcost_G(A(G))] \leq \dcost_G^* + K \frac{n^2}{\epsilon}$ for some constant $K$.

Our graphs will make use of expander graphs, which have the following definition
\begin{defn}
A $D$-regular, $n$-vertex undirected graph is a $\lambda$-expander if $\lambda_2(G) \leq \lambda$.
\end{defn}
There exist explicit constructions of $D$-regular Ramanujan graphs which satisfy $\lambda_2(G) \leq 2\sqrt{D-1}$. For our purposes, we will consider random $D$-regular graphs.
\begin{thm}
For any $D,n$, a random $D$-regular (undirected) graph satisfies $\lambda_2(G) \leq 2\sqrt{D-1} + O(1)$.
\end{thm}

The next theorem will allow us to link spectral expanders to vertex expanders.

\begin{thm} (Expander Mixing Lemma)
Let $G$ be a $D$-regular, $N$-vertex digraph such that $\lambda_2(G) = \lambda D$ for $\lambda \geq 0$. For any sets $S,T \subseteq V$ with $\alpha = \frac{|S|}{N}$ and $\beta = \frac{|T|}{N}$, we have
\[
    \left|\frac{w_G(S,T)}{ND} - \alpha \beta\right| \leq \lambda \sqrt{\alpha (1-\alpha)\beta(1-\beta)}
\]
\end{thm}

Now, we tightly characterize the cost of any hierarchical clustering of $G$:
\begin{lem}
    Let $G$ be a $D$-regular, $N$-vertex graph with $\lambda_2(G) = \lambda D$. Let $R \subseteq V$ be a subset of the vertices with $|R| = r$, and $G[R]$ be the induced subgraph of $G$. Then, $r^2 D (\frac{4r}{27N} - \frac{\sqrt{8}}{9}\lambda) \leq \dcost_{G[R]}^* \leq r^2D(\frac{r}{3N} + \lambda)$.
\end{lem}
\begin{proof}
    First, consider the cost of a perfectly-balanced HC graph. At level $i$ for $i = 0, \ldots, \log r$, there are $2^i$ subtrees, each of size $\frac{r}{2^i}$. Each subtree cuts the vertices into two pieces $S_1, S_2$ of size $\frac{r}{2^{i+1}}$. Applying the expander mixing lemma, we have 
    \begin{align*}
        w_{G[R]}(S_1, S_2) &\leq \frac{|S_1||S_2|}{N^2} ND + \lambda ND\sqrt{\frac{|S_1||S_2|}{N^2}} \\
        &\leq \frac{r^2}{2^{2i+2}N}D + \lambda D \frac{r}{2^{i+1}}.
    \end{align*}
    Therefore, the total cost of a balanced tree $B$ is
    \begin{align*}
        cost_{G[R]}(B) &= \sum_{i=0}^{\log r} 2^i \frac{r}{2^i} \left( \frac{r^2}{2^{2i+2}N}D + \lambda D \frac{r}{2^{i+1}} \right) \\
        &= \frac{r^3 D}{N} \sum_{i=0}^{\log r} \frac{1}{2^{2i+2}} + \lambda D r^2 \sum_{i=0}^{\log r} \frac{1}{2^{i+1}} \\
        &\leq r^2D(\frac{r}{3N} + \lambda).
    \end{align*}
    
    Define $f(s) = \min_{S \subset V, |S| = s} \dcost_{G[S]}^*$. We have $f(1) = 0$. Let $T$ be any tree on $R$ with $T = S_1 \cup S_2$ such that $|S_1| = s_1$ and $|S_2| = s_2$. By the Expander mixing lemma, we have
    \[
        w_{G[R]}(S_1, S_2) \geq \frac{s_1s_2}{N} D - \lambda D\sqrt{s_1s_2} \\
    \]
    This is the cost incurred by the initial split of any tree on a subset $S$. Thus, we have
    \[
        f(s) \geq \min_{s_1 + s_2 = s} f(s_1) + f(s_2) + s\left(\frac{s_1s_2D}{N} - \lambda D \sqrt{s_1 s_2}\right)
    \]
\end{proof}

\begin{theorem}

\end{theorem}

\begin{defn}
For a set $S \subseteq V$ with $\frac{n}{3} \leq |S| \leq \frac{n}{2}$, define the approximate matching graph $\calH(S)$ to be a graph in which the first $\frac{n}{2} - |S|$ elements of $S$ are matched with the first $2$ available unmatched vertices in $V \setminus S$, and the remaining vertices are matched with the first available unmatched vertex in $V$.
\end{defn}
\begin{obs}
For any balanced cut $S$, $\dcost_{K_S}^* \leq 3n$.
\end{obs}
\begin{proof}
$K_S$ consists of $|S| \leq \frac{n}{2}$ connected components of sizes between $2$ and $3$. Any hierarchical clustering which preserves these components until the last split incurrs at most cost $5$ cost per component.
\end{proof}
Approximate matching graphs form the adversarial set of graphs used in our lower bound. Next, consider the following way of partitioning the leaves of a Hierarchical clustering:
\begin{defn}
For a binary hierarchical clustering $T \in \calT_n$, define the balanced split to be the following: Let $T = split(T_1, split(T_2, \ldots, split(T_{k-1}, T_k)))$, where $|T_i| \leq \frac{n}{3}$ for $1 \leq i \leq k-1$, and $\frac{n}{3} \leq T_k \leq \frac{2n}{3}$. The balanced split of $T$ is the split $(U, V) = (T_k, T_1 \cup \cdots \cup T_{k-1})$.
\end{defn}
\begin{obs}
Let $(U,V)$ denote the balanced split of $T$. Let $G$ be an arbitrary graph. Then, $\dcost_G(T) \geq \frac{n}{3} w_G(U,V)$.
\end{obs}
\begin{proof}
Any edge of $G$ that cuts $U,V$ is part of a subtree which is size at least $\frac{n}{3}$, as $U$ is part of the subtree and has size at least $\frac{n}{3}$.
\end{proof}

If the balanced split of a tree differs greatly from the set $S$, then the tree will incur a high cost on $\calH(S)$.
\begin{lem}
Let $T \in \calT_n$ be a hierarchical clustering with balanced split $(U,V)$. Let $S$ denote a balanced cut. Then, 
\[
    \dcost_{\calH(S)}(T) \geq \min\{d_H(S, U), d_H(S, V)\} n,
\]
where $d_H$ denotes the Hamming distance.
\end{lem}
\begin{proof}
From our observation, we have $\dcost_{\calH(S)}(T) \geq w_{\calH(S)}(U,V)\frac{n}{3}$. 
\end{proof}
\fi 

\iffalse
\section{Omitted Details from HSBM}

\iffalse 
\begin{thm}\label{thm:SBM-recovery}
(Theorem 12 from~\cite{mcsherry2001spectral}): Let $\sigma = \max_{i,j} \sqrt{A_{ij}(1-A_{ij})}$, and suppose this value is at least $\frac{\log^3(n)}{\sqrt{n}}$. Let $s = \min_{i=1}^k |B_i|$. Split the columns of $\hat{A}$ into two equal pieces $\hat{A}_1$ and $\hat{A}_2$. Define $P_1, P_2$ to be projection operators given by $P_1 = SVD_k(\hat{A}_1)$ and $P_2 = SVD_k(\hat{A}_2)$ If $i$ is a column in $\hat{A}$, then let $\zeta(i) = P_1((\hat{A}_2)_i$; otherwise let $\zeta(i) = P_2((\hat{A}_1))_i$. The following holds for all $1 \leq i \leq \frac{n}{2}$ with probability at least $1-\frac{1}{n^6}$:
\begin{align*}
    \|A_i - \zeta(i)\|_2 \leq 8 \sigma \sqrt{\tfrac{nk}{s}} + \sqrt{10k \log n}
\end{align*}
\end{thm}

\ji{JI: The McSherry paper seems to require only one of the blocks in the SBM to be at least $\frac{\log^3(n)}{\sqrt{n}}$. This is quite a weak requirement. Still, when it is not possible, there is another theorem that allows for results with smaller $\sigma$. This could allow us to do away with this requirement.}

This allows us to derive the following:

\begin{coro}
    For an HSBM $(P,f)$ with label function $\psi : V \rightarrow [k]$ and adjacency matrix $A$, suppose that $\|A_i - A_j\|_2 \geq 5\Delta$ for all $i,j$ such that $\psi(i) \neq \psi(j)$, where $\Delta = 8 \sigma \sqrt{\tfrac{nk}{s}} + \sqrt{10k \log n}$. We have that $\|\zeta(i) - \zeta(j)\|_2 \geq 3\Delta$ for all $i,j$ such that $\psi(i) \neq \psi(j)$, and $\|\zeta(i) - \zeta(j)| \leq 2\Delta$ for all $i,j$ such that $\psi(i) = \psi(j)$.
\end{coro}

The corollary shows that exact recovery is possible, and when we are able to perform exact recovery of $\psi$ using clustering, we can essentially compute the HC exactly. 


\subsection{Applying the above with randomized response}

To begin to do recovery with privacy, suppose we are given an adjacency matrix $A$ in the HSBM with parameters $(P,f)$ such that $\|A_i - A_j\|_2 \geq C$ when $\psi(i) \neq \psi(j)$. Normally, the input graph has adjacency matrix $\hat{A}$, but even this graph is private information. To make it satisfy differential privacy, we apply randomized response to $\hat{A}$ with parameter $\rho = \frac{1}{e^\epsilon + 1}$. This gives us the graph $\hat{B}$ which is a randomized rounding of the matrix $B = A * \rho$, where $x * \rho = x (1-\rho) + (1-x) \rho$. 

The block sizes of $B$ are the same as those of $A$, and the maximum variance $\sigma_B$ of the elements of $B$ is at least at least as high as $\sigma_A$, and it must be at least $\rho$. Finally, substituting $B_i = A_i(1-2\rho) + \rho \textbf{1}$, we have
\[
    \|A_i - A_j\|_2 = (1-2\rho)\|B_i - B_j\|_2.
\]
To apply Corollary 1 to $B$ and perform recovery, we need the minimum distance $C$ to be at least $\frac{1}{1-2\rho}\left(8 \sigma_B \sqrt{\frac{nk}{s}} + \sqrt{10k \log n}\right)$.
\fi 
\fi
